# Supplementary material for: Effective Monitoring of Online Decision-Making Algorithms in Digital Intervention Implementation
Source: arXiv:2409.10526 source file (2024-08-30)
Supplement: Supplementary file 1 [file a.tex]

\section{Terminologies we can think to use}
\begin{itemize}
    \item SDV - Source Data Verification. Source Data Verification (SDV) is a method that clinical research organizations can use to ensure the data they're collecting is accurate. Source data verification is an essential tool for ensuring the quality of your clinical trial data. Read more \href{https://vial.com/blog/articles/clinical-trial-basics-source-data-verification-sdv/?https://vial.com/blog/articles/clinical-trial-basics-source-data-verification-sdv/?utm_source=organic}{here}.
    
\end{itemize}

\section{Software System Components}
\alt{Need to think more carefully about if we should keep this section or if Section 3.1 General Software Framework already covers this.}
\alt{If we do keep, Anna needs to change all the language to be less RL and consistent with the clinical language in the main paper}
\sg{We can chuck it now? Or maybe just define terms specific for understanding the appendix}
\subsection{Definitions}
\begin{itemize}
    \item Endpoint
\end{itemize}

\subsection{Oralytics Software System Components}
\label{sec_system_components}
The RL algorithm is one component of the RL software service. The RL service consists of (1) an API to communicate with other services, (2) a dependency module to request sensor data from other services, (3) a module to update the RL algorithm based on newly collected participant data, (4) an action-selection module that takes in the participant's current state and assigns an intervention based on the algorithm's current policy, and (5) an internal database that stores all the data necessary for the RL algorithm to function and perform post-trial analyses. 

To function properly, the RL service depends on stable interactions with a variety of other services. We refer to this larger ecosystem of software components as the digital intervention software system (Figure~\ref{fig:digital_interventions_arch}). The sensor collection device collects relevant sensor data (e.g., brushing data or app analytics data) that is used in state and/or reward construction for the RL algorithm. For each participant's decision time, the backend main controller collects sensor data, makes this data available for the RL service to request, and calls the RL API's action selection module. Once called, the RL service obtains the recent sensor data, constructs the participants' state features, then returns the actions selected by the RL algorithm's policy. The RL service saves the necessary data corresponding to the state and action to the internal database.
%to receive the actions selected according to the RL algorithm's policy, 
The backend main controller then scheduled prompts accordingly. During algorithm update time, the backend main controller collects sensor data needed for reward construction from the commercial cloud, makes this data available for the RL service to request, and calls the RL API's algorithm update module. The RL service obtains the recent sensor data, constructs rewards for each new decision-time, and then updates its policy using the entire history of state, action, and reward data. The RL service saves the necessary data corresponding to reward and policy to the internal database. As one can see, proper RL algorithm functionality requires frequent real-time communication between a variety of components. While the trial is running, many things could go wrong.

%%% ORALYTICS DIAGRAM %%%
\begin{figure*}[t]
    \centering
    \includegraphics[trim={1.1cm 1.5cm 1.4cm 3.8cm},clip,width=0.8\textwidth]{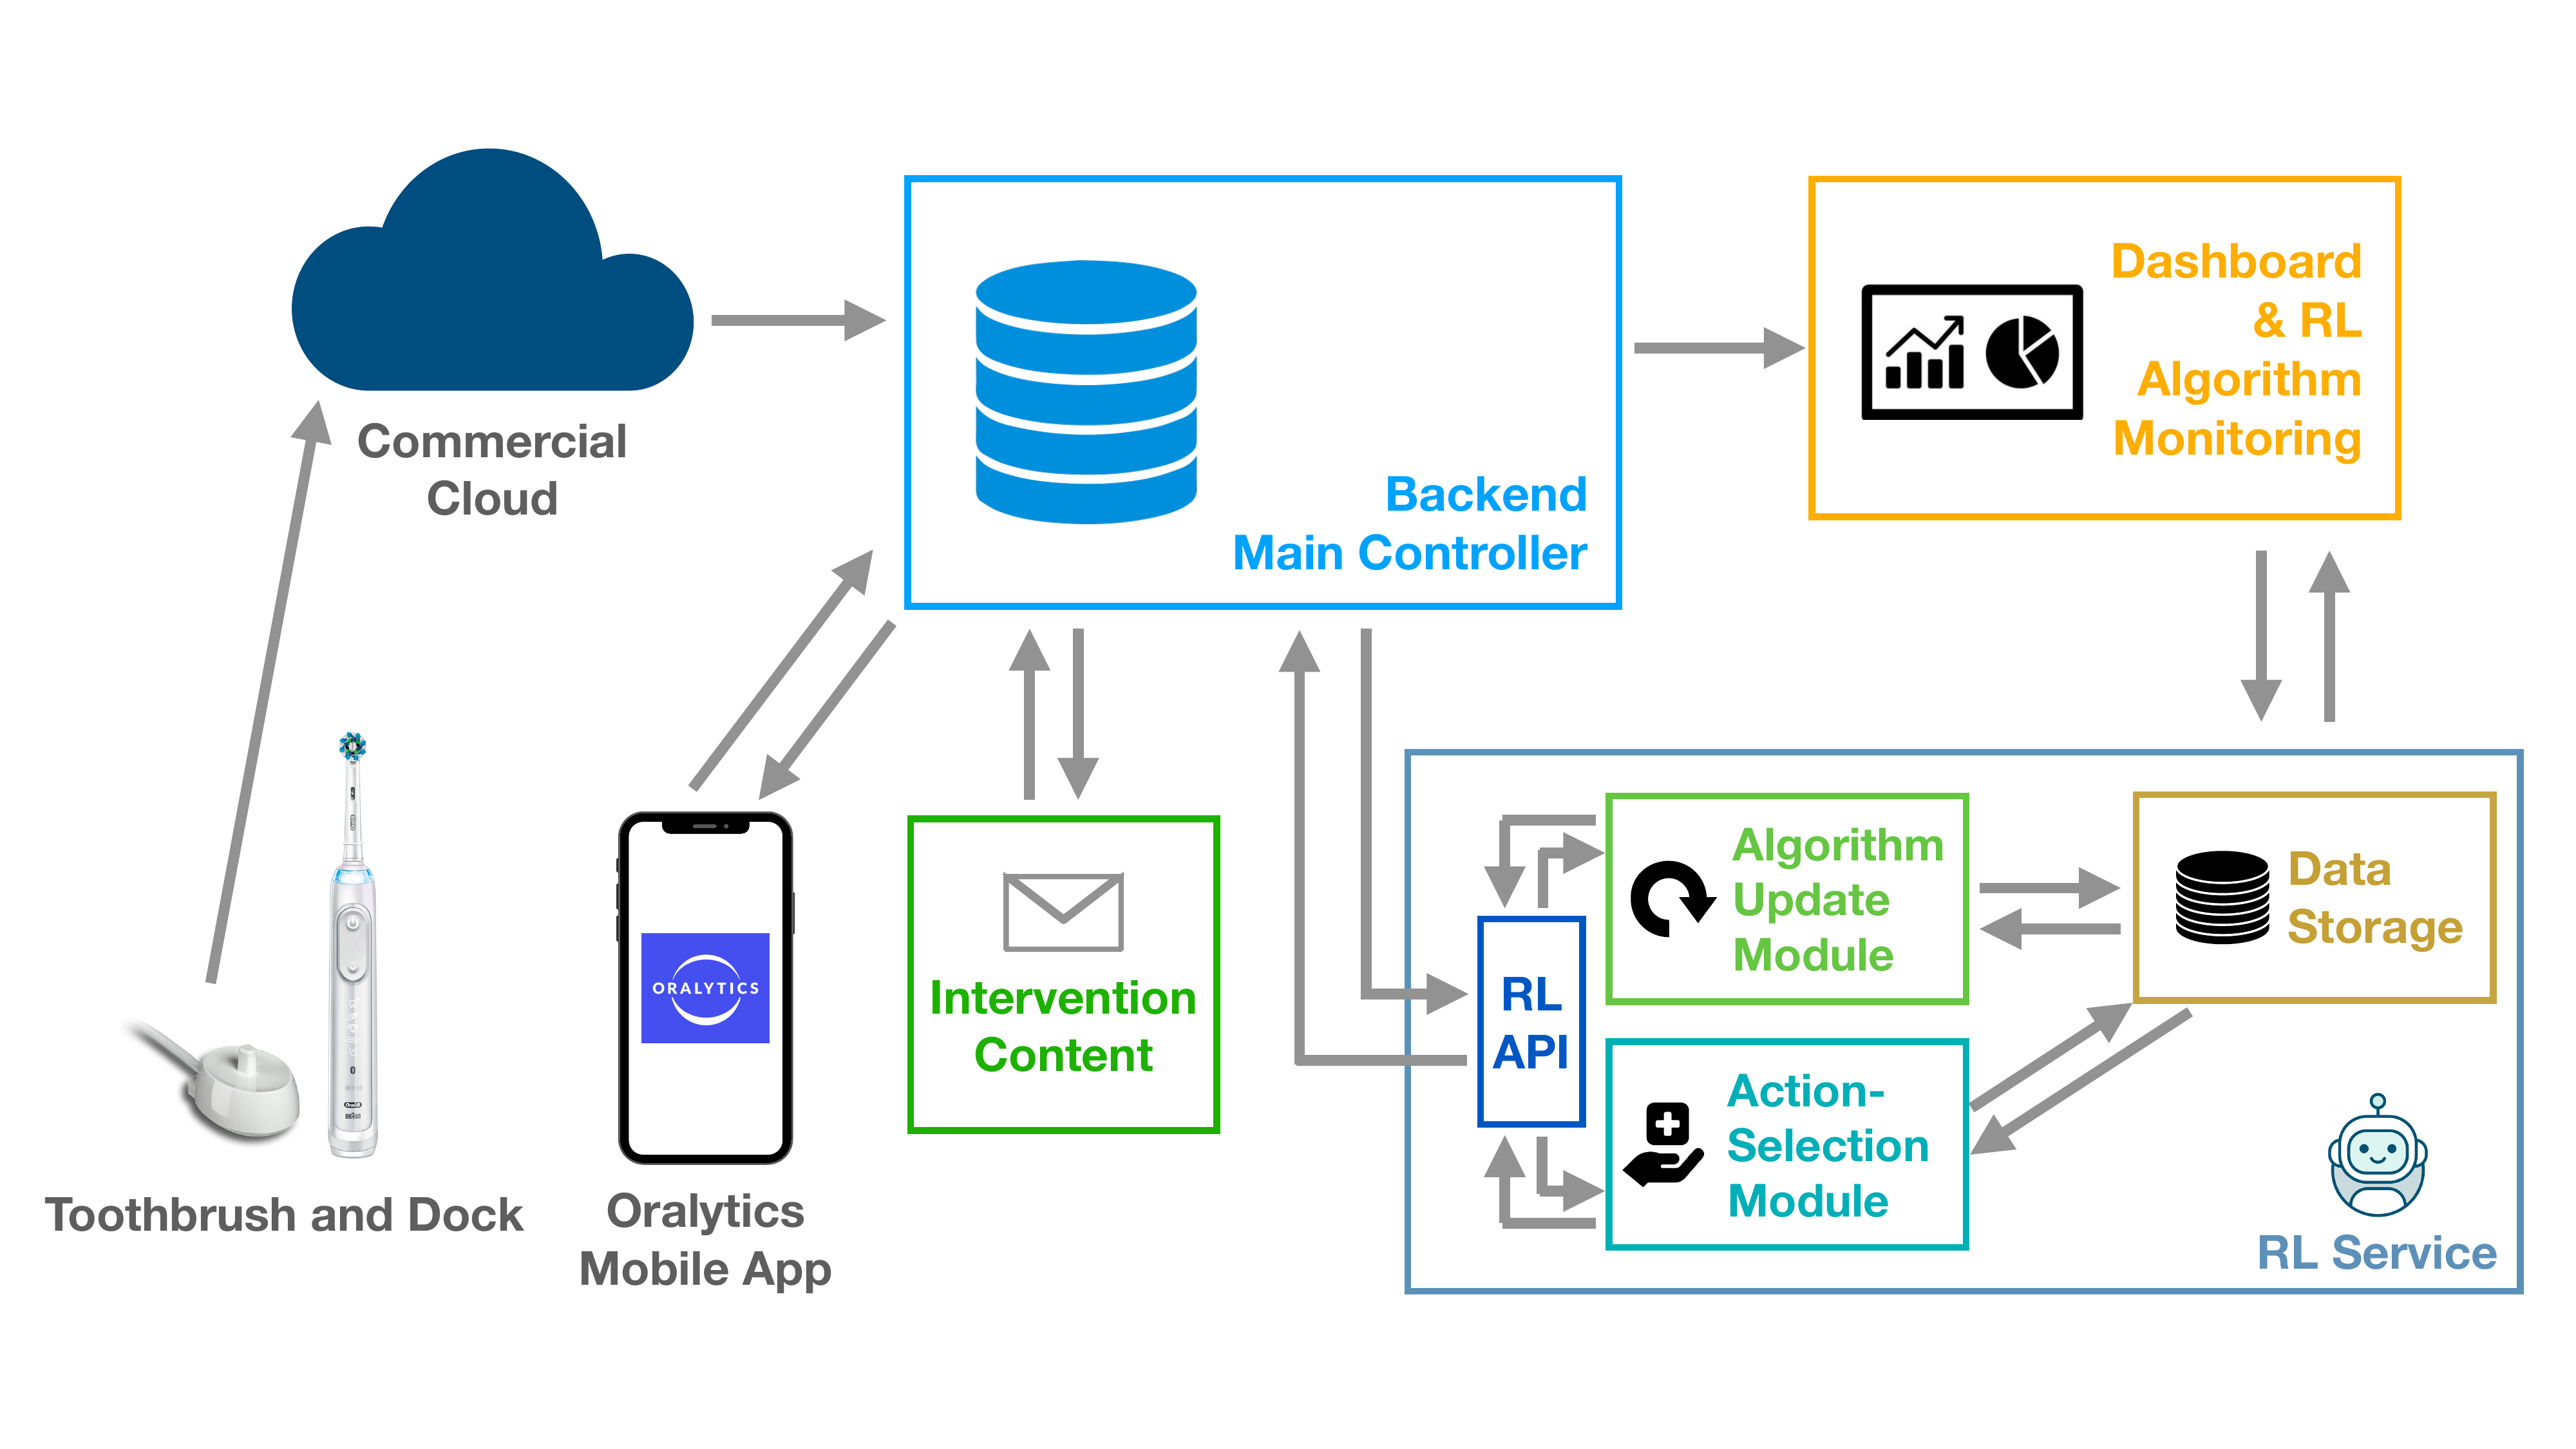}
    \caption{Oralytics System and RL System Architecture. Brushing data is captured by sensors in the toothbrush and uploaded to the commercial cloud via a dock. The main controller gathers this data, along with app engagement data from the Oralytics app, and feeds it to the RL service and the dashboards. This sensor data is provided to the RL service to select actions and update. Using the actions selected by the RL service, the main controller populates intervention prompt content, and schedules prompts onto each participant's Oralytics app.}
    \label{fig:oralytics_architecture}
\end{figure*}
