# Supplementary material for: Effective Monitoring of Online Decision-Making Algorithms in Digital Intervention Implementation
Source: arXiv:2409.10526 source file (2024-08-30)
Supplement: Supplementary file 2 [file other_fidelity.tex]

\section{Additional Forms of Fidelity}
\label{app_other_forms_fidelity}
In this paper, we focus mainly on RL algorithm fidelity; however, there can be other types of fidelity that are important to consider when running an online algorithm in a clinical trial. In addition to algorithm fidelity, there is also \textit{system fidelity} (i.e., how each component in the clinical trial works together) and \textit{participant fidelity} (i.e., participant adherence when participating in the trial). System fidelity can involve verifying correct communication between the sensory-collection device, the data storage system, the computation system where the algorithm runs, and the device that administers the action. Notice that algorithm fidelity is part of system fidelity. On the other hand, participant fidelity can involve concerns such as ensuring the participants are able to correctly download or update the app, keep their smart device charged, actions needed from the participant to obtain sensory data, etc. We make the distinction that issues can arise that impact post-trial analyses and participant experiences that are caused by other components of the system failing (e.g., expired credentials cause participants to lose access to the mobile app), however, this paper focuses on issues that are directly controlled or caused by the RL algorithm.

% \sam{in clinical trials, a big issue is fidelity to the intervention/treatment schedule.  I think this likely comes under system fidelity except people in clinical trials don't use the phrase "system fidelity."  We will need help from Billie here.  For example usually contact between the clinical staff providing a behavioral treatment is protocolized and the protocol is published ahead of time.  This is to ensure that all participants randomized to a treatment receive the same treatment.  An example in our case, is when there is a mix of smartphones, like ios and android.  These phones may display intervention messages/feedback differently and thus have differing effects.   Scientists plan ahead for this by recording the phone type along with other pretreatment variables and then use this feature in after study analyses. Another big issue in trials of medicines is blinding the participant and the clinical staff to the treatment the participant is assigned to.  The CITI exams also likely provided references to good cites for this.  I'm not sure whether we should discuss this here.   Just listing all the other forms of fidelity might take up too much room... }
